# Supplementary material for: Electric Autonomous Mobility-on-Demand: Jointly Optimal Vehicle Design and Fleet Operation
Source: arXiv:2309.13012 source file (2023-09-21)
Supplement: Supplementary file 1 [file Appendix.tex]

\appendices
\section{List of Variables}
\label{Sec:app}
The variables used to formulate Problem~\ref{prob:main} are defined as follows:
\begin{itemize}
\item{$X \in \{0,1\}^{\abs{\cI^+} \times \abs{\cI^+} \times K}$: binary variable representing if transition between request $i$ and $j$ is served by vehicle $k$.}
\item{$S\in \{0,1\}^{\abs{\cI^+} \times \abs{\cI^+}\times C \times K}$: binary variable indicating if charging occurs at station $c$ during $i$ to $j$ transition, served by vehicle $k$.}
\item{$C\in \mathbb{R+}^{\abs{\cI^+} \times \abs{\cI^+} \times C \times K}$: continuous variable representing energy charged by vehicle $k$ between $i$ and $j$ at station $c$, in kWh.}
\item{$E\in \mathbb{R+}^{\abs{\cI^+} \times \abs{\cI^+}\times K}$: continuous variable indicating energy spent to go from $i$ to $j$ and serve $j$, in kWh.}
\item{$e\in \mathbb{R+}^{\abs{\cI^+} \times K }$: continuous variable representing energy stored by vehicle $k$ after serving request $i$, in kWh.}
\item{$E_\mathrm{b}\in \mathbb{R+}^{K}$: continuous variable representing the maximum energy stored by vehicle $k$ during simulation, in kWh.}
\item{$b_\mathrm{v}\in \{0,1\}^{K}$: binary variable indicating if vehicle $k$ is active.}
\item{$b_\mathrm{r}\in \{0,1\}^{\abs{\cI^+}}$: binary variable indicating if request $i$ is served .}
\item{$f\in \{0,1\}^{\abs{\cI^+} \times K}$: binary parameter used to initialize vehicle $k$ in the depot, with 1 indicating $j$ is starting depot.}
\item{$l\in \{0,1\}^{\abs{\cI^+} \times K}$: binary parameter used to finalize vehicle $k$ in the depot, with 1 indicating ending depot.}
\end{itemize}
Note: $b_\mathrm{v}$ can be made an integer variable to accommodate multiple types of vehicles. If free floating fleets are used, $f$ and $l$ can be considered as optimization variables. If depots are present, they are used to initialize/finalize vehicles.

\section{Sampling Error}\label{sec:error}
In this section, we analyze the impact that the sample size has on the distribution of the travel requests. %from a probabilistic point of view to show that a sampling error might be induced, especially in smaller scenarios. %Intuitively, when we sample the set of travel requests, if the number of requests is underestimated, the vehicles idle more, not being able to serve potential requests; if the requests are overestimated, either more vehicles are required to serve them, or the rejection rate increases. 
In a strongly simplified scenario, given a large set of travel requests $\cI$, if all the requests must be served, the lower bound of the number of vehicles is equal to the maximum number of requests that occur simultaneously. Because of the stochastic nature of the phenomenon, it is useful to estimate the probability for a certain number of requests to be simultaneous. 
Such a probability of overlapping events can be found by modeling the starting times of the events as a uniform distribution in the time window $T_{\mathrm{w}}$, and using a binomial distribution~\cite{DekkingKraaikampEtAl2005} to model the number of overlapping events~\cite{Thomas1988}.
Specifically, let $n$ be the number of occurrences of the event at time window $T_{\mathrm{w}}$, and let $T_\mathrm{avg}$ be the average time of duration of the event. Assuming the starting time is uniformly distributed in the time window $T_{\mathrm{w}}$, the probability of overlapping $k$ times is given by
\begin{equation}\label{eq:probab}
	P(n,k) = \binom{n}{k} \left( \frac{T_\mathrm{avg}}{T_{\mathrm{w}} } \right)^k  \left(1 - \frac{T_\mathrm{avg}}{ T_{\mathrm{w}} } \right)^{n-k}.
\end{equation}
For a small time-window, e.g., a few hours of rush hour, it is reasonable to estimate the probability of the starting time of the events to be uniform. 
Fig.~\ref{fig:prob} depicts the probability distribution described in~\eqref{eq:probab}, with $\abs{\cI} = 1000$ travel requests during a peak-time of $\unit[3]{h}$.  
\begin{figure}[t]
	\centering
	\includegraphics[trim={0cm 1 10 10},clip,width=\linewidth]{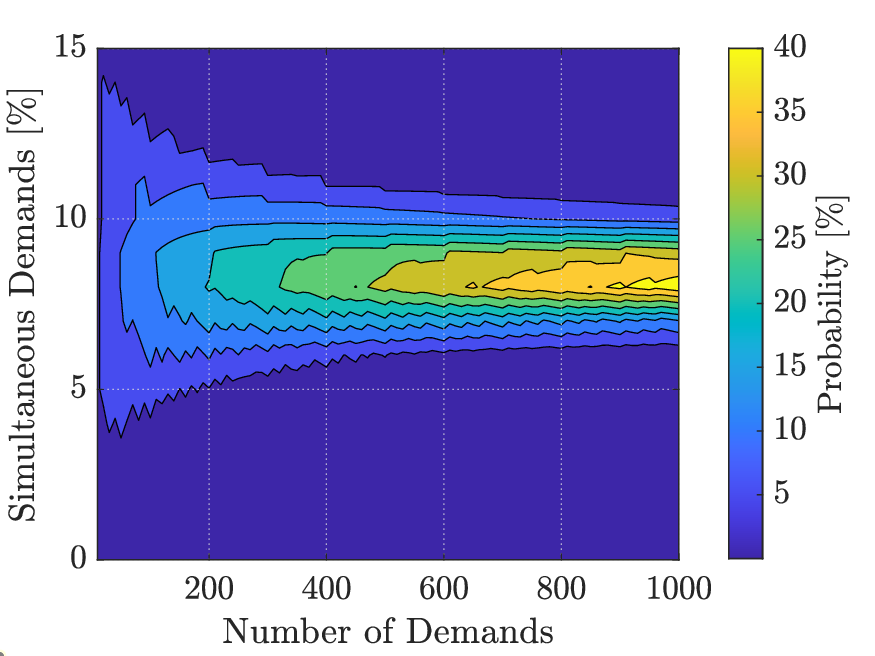}
	\caption{Probability of overlapping events as a function of simultaneous travel requests and overall number of events. The time window is $T_{\mathrm{w}}=\unit[3]{h}$, while $T_\mathrm{avg}=\unit[0.25]{h}$.}
	\label{fig:prob}
\end{figure} 
Thereby, we observe that by sampling from the distribution, the mean remains the same, whilst the measured variance increases for lower number of demands.
Therefore, when solving for smaller scenarios, we can expect to be solving problems that are on average similar, but that display a larger variance compared to larger scenarios. In turn, we speculate the solution's distribution to also have a larger variance, which should be accounted for when choosing the extent to which a design solution is conservative.
%For this reason, by samplings the distribution multiple times, the goal is to obtain a distribution with the same mean value. 
%However, because of the higher variance, some scenarios will require a larger number of vehicles. 
%In addition, as shown in Section~\ref{sec:size}, the sampling size itself influences the quality of the solution. Ultimately, the size of the scenarios should be maximized w.r.t. the available time and computational resources.
